# Supplementary material for: Self-consistency in $GW\Gamma$ formalism leading to quasiparticle-quasiparticle couplings
Source: arXiv:2203.05029 ancillary file (2022-08-09)
Supplement: Supplementary file 1 [file Correlation_Vertex.pdf]

# Supporting information for "Self-consistency in $GW\Gamma$ formalism leading to quasiparticle-quasiparticle couplings"

Carlos Mejuto-Zaera* and Vojtěch Vlček†
*University of California, Santa Barbara*
(Dated: August 9, 2022)

In this Supporting Information (SI) we include

1. A note on the resummation of the equation for $\frac{\delta W}{\delta G}$.
2. Derivation of Hedin's equations in orbital space.
3. Concrete expressions for the perturbative approximations implemented in the main paper.
4. Comments on the mean-field approximation on the Hubbard dimer.
5. Simulation parameters to reproduce the results in Fig. 3 of the main paper.
6. Attached file with the data in Fig. 3 of the main paper.

## I. ON THE RESUMMATION OF $\frac{\delta W}{\delta G}$

In the main paper, and particularly in Fig. 1, we show that the leading contributions from $\frac{\delta W}{\delta G}$ and $\frac{\delta \Gamma}{\delta G}$ to the interaction Kernel are asymmetric in the appearance of unscreened/screened interaction lines. In particular, the leading term in $\mathcal{K}_W \propto \frac{\delta W}{\delta G}$ includes an unscreened interaction line at the end of the "$T$-matrix box", while the corresponding exchange diagram from $\mathcal{K}_\Gamma$ presents screened interactions lines throughout. In this note, we show how the final unscreened interaction line in $\mathcal{K}_W$ gets dressed by performing a Dyson-type resummation of the most general equation for $\frac{\delta W}{\delta G}$. By doing this, we will further cement the central message of the main paper: that topological novel diagrams are exclusively introduced by $\frac{\delta \Gamma}{\delta G}$, which we used to argue for the fundamental relevance of the $\mathcal{K}_\Gamma$ kernel in pushing the validity of Hedin's based MBPT towards high interactions.

In real space, the equation determining the screened interaction $W$ is a Dyson-like recursive equation involving the bare interaction $v$ and the polarization function $P(1,2)$, which follows [1, 2]

$$W(1,2) = v(1,2) + v(1,\bar{3})P(\bar{3},\bar{4})W(\bar{4},2), \tag{1}$$

where the usual short hand notations $(1) \equiv \{\vec{r}_1, t_1, \sigma_1\}$ and $A(\bar{1})B(\bar{1}) \equiv \sum_{\sigma_1}\int \mathrm{d}\vec{r}_1 \mathrm{d}t_1\ A(\vec{r}_1,t_1,\sigma_1)B(\vec{r}_1,t_1,\sigma_1)$ are employed, and we write the local, instantaneous bare Coulomb interaction as $v(1,2) = \delta(t_1 - t_2)\frac{1}{|\vec{r}_1 - \vec{r}_2|}$. We can take the functional derivative with respect to $G$ to find

$$\frac{\delta W(1,2)}{\delta G(5,6)} = v(1,\bar{3})\frac{\delta P(\bar{3},\bar{4})}{\delta G(5,6)}W(\bar{4},2) + v(1,\bar{3})P(\bar{3},\bar{4})\frac{\delta W(\bar{4},2)}{\delta G(5,6)}. \tag{2}$$

This is, again, a Dyson-type recursive equation, this time for $\frac{\delta W}{\delta G}$. We can sketch its solution iteratively, by substituting order by order the first half of the RHS of the equation in the final $\frac{\delta W}{\delta G}$ term. This gives, omitting the integral indices for simplicity

* carlos_mejutozaera@ucsb.edu, current: cmejutoz@sissa.it
† vlcek@ucsb.edu

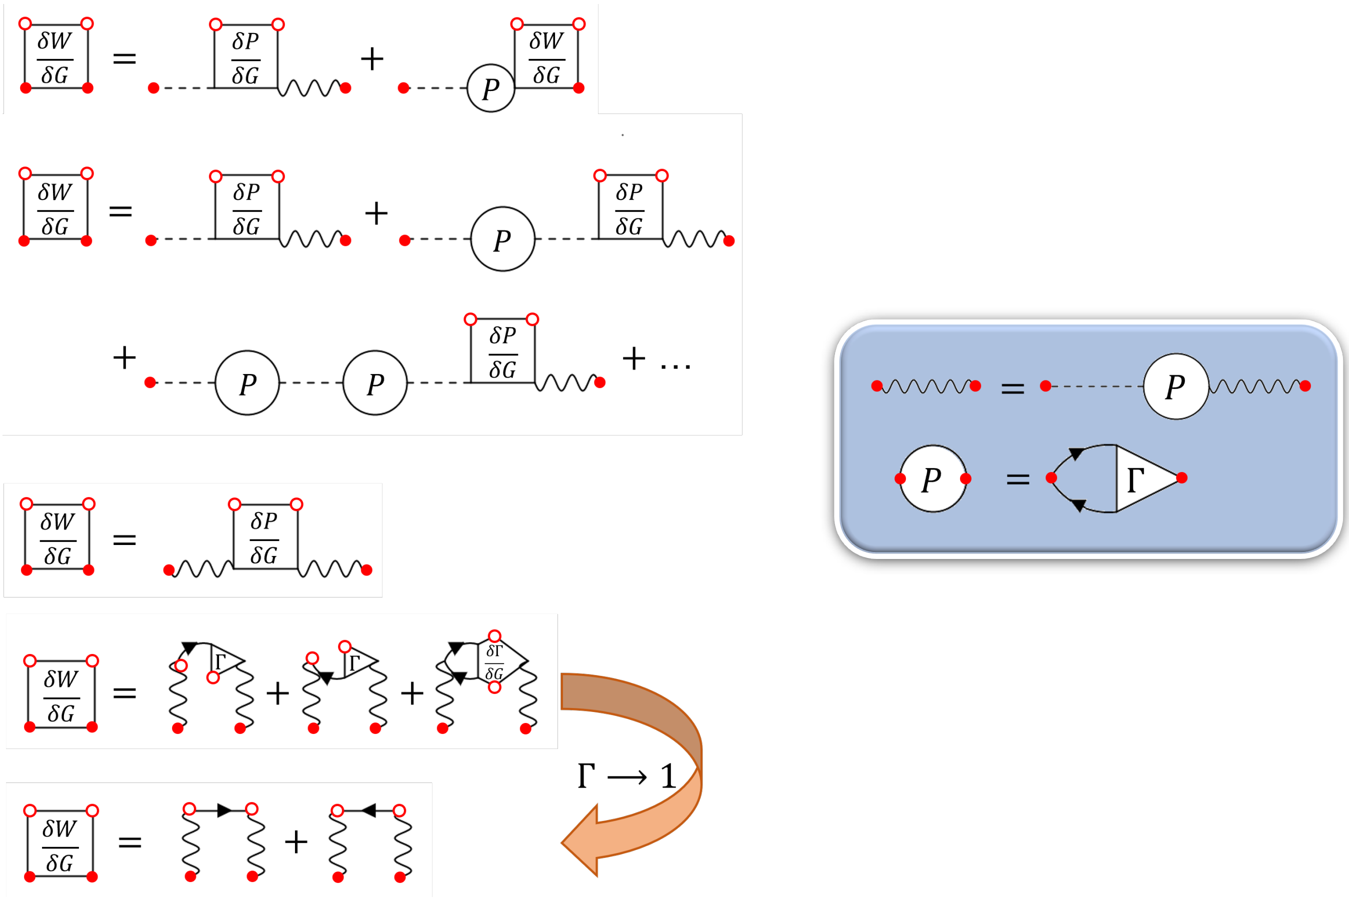


FIG. 1. Diagrammatic derivation sketch of $\delta W/\delta\Gamma$. In the last line, the limit $\Gamma \to 1$ is taken. The external legs of each diagram are marked with dots. External legs for $W$ or $P$ are marked as solid dots, those coming from the functional derivative with respect to $G$ are represented as empty dots. The pentagon in the fifth line represents the functional derivative of $\Gamma$ with respect to $G$.

$$
\begin{aligned}
\frac{\delta W}{\delta G} &= v\frac{\delta P}{\delta G}W + vP\frac{\delta W}{\delta G}, \\
&= v\frac{\delta P}{\delta G}W + vPv\frac{\delta P}{\delta G}W + vPvPv\frac{\delta P}{\delta G}W + \cdots, \\
&= (v + vPv + vPvPv + \cdots)\frac{\delta P}{\delta W}W, \\
&= W\frac{\delta P}{\delta W}W.
\end{aligned} \tag{3}
$$

In the last line we have identified $W = v + vPv + vPvPv + \cdots$ as the formal solution to the $W$ Dyson equation in Eq. (1). Now, the leading term in $\mathcal{K}_W$ discussed in the main paper corresponds to the first term in the second line of Eq. (3), which indeed has an unscreened $v$ line and a screened $W$ line. The exact expression for $\frac{\delta W}{\delta G}$ can be obtained by substituting this bare interaction line by a screened one. We present a pictorial sketch of the derivation in Fig. 1

Now, we can note that the diagrams entering $\frac{\delta W}{\delta G}$ are essentially identical to those composing $\frac{\delta P}{\delta G}$, plus two external $W$ lines. The polarization can be written as $P = -iGG\Gamma$ (see Ref. [1] or Ch. 10 and 11 in Ref. [2]). Hence, just like we saw in the main paper for the interaction kernel, non-trivial diagrams can only be generated by $\frac{\delta\Gamma}{\delta G}$. If we only keep its trivial component, leading to the RPA approximation $P = -iGG$, the $\frac{\delta W}{\delta G}$ will exclusively contain the first order direct $T$-matrix terms discussed in the main paper (c.f. last line in Fig. 1). Hence, even if arguably both $\mathcal{K}_W$ and $\mathcal{K}_\Gamma$ contain non-trivial functional derivatives with respect to $G$ ($\frac{\delta W}{\delta G}$ and $\frac{\delta\Gamma}{\delta G}$ respectively), it is fundamentally only the derivative in the latter, the derivative of the interaction vertex $\Gamma$, the one that can introduce topologicaly new diagrams beyond the $GW\Gamma_x$ (see Refs. [3–5]) and direct $T$-matrix approximations. This further underlines the

central role of $\mathcal{K}_\Gamma$ (in particular $\frac{\delta\Gamma}{\delta G}$) in pushing many-body perturbation theory beyond the weakly-interacting limit.

## II. HEDIN'S EQUATIONS IN ORBITAL SPACE

To implement Hedin's equations [1] for a model lattice Hamiltonian, such as the Hubbard model, it is advantageous to change from the traditional representation in real space (cf. Ref. [6]) to orbital space. While writing this paper, it proved unexpectedly difficult for us to find references in the literature containing Hedin's equations in an orbital basis, with the exception of one appendix in Ref. [2]. Hence, we want to provide and derive these equations here.

Writing Hedin's equations in orbital space corresponds to using as basis for the single-particle states some complete set of orbitals $\phi_{a,\sigma}(\vec{r})$ instead of the real-space field operators $\psi^\dagger_\sigma(\vec{r})$. These two bases are related by

$$\psi^\dagger_\sigma(\vec{r}) = \sum_a \phi_{a,\sigma}(\vec{r}) c^\dagger_a, \tag{4}$$

where $\sigma$ represents the particle spin, and $a$ is a collective label for all other quantum numbers necessary to completely identify a single-particle state, and $c^\dagger_a$ corresponds to the creation operator for an electron in orbital $\phi_a(\vec{r})$. Both $\psi^\dagger_\sigma(\vec{r})$ and $c^\dagger_{a,\sigma}$ obey the common Fermionic anti-commutation relations

$$\left\{\psi^\dagger_\sigma(\vec{r}), \psi^\dagger_{\sigma'}(\vec{r'})\right\} = \left\{\psi_\sigma(\vec{r}), \psi_{\sigma'}(\vec{r'})\right\} = 0, \left\{\psi^\dagger_\sigma(\vec{r}), \psi_{\sigma'}(\vec{r'})\right\} = \delta_{\sigma,\sigma'}\delta(\vec{r}-\vec{r'}), \tag{5}$$

$$\left\{c^\dagger_{a,\sigma}, c^\dagger_{b,\sigma'}\right\} = \{c_{a,\sigma}, c_{b,\sigma'}\} = 0, \{c^\dagger_{a,\sigma}, c_{b,\sigma'}\} = \delta_{\sigma,\sigma'}\delta_{a,b}. \tag{6}$$

In the real space basis, Hedin's equations read (cf. Ref. [6] or Ch. 10 and 11 in Ref. [2])

$$\Gamma(1,2;3) = \delta(1,2)\delta(1,3) + \frac{\delta\Sigma_{xc}(1,2)}{\delta G(\bar{4},\bar{5})} G(\bar{4},\bar{6})G(\bar{7},\bar{5})\Gamma(\bar{6},\bar{7};3), \tag{7}$$

$$P(1,2) = -iG(2,\bar{3})G(\bar{4},2)\Gamma(\bar{3},\bar{4};1), \tag{8}$$

$$W(1,2) = v(1,2) + v(1,\bar{3})P(\bar{3},\bar{4})W(\bar{4},2), \tag{9}$$

$$\Sigma(1,2) = \Sigma_H(1,2) + iW(1^+,\bar{3})G(1,\bar{4})\Gamma(\bar{4},2;\bar{3}), \tag{10}$$

$$G(1,2) = G^0(1,2) + G^0(1,\bar{3})\Sigma(\bar{3},\bar{4})G(\bar{4},2), \tag{11}$$

where, as above, the usual short hand notations $(1) \equiv \{\vec{r}_1, t_1, \sigma_1\}$ and $A(\bar{1})B(\bar{1}) \equiv \sum_{\sigma_1}\int \mathrm{d}\vec{r}_1 \mathrm{d}t_1\; A(\vec{r}_1,t_1,\sigma_1)B(\vec{r}_1,t_1,\sigma_1)$ are employed, and a + superscript over a variable symbolizes the limit $A(x^+) \equiv \lim_{\eta\to 0^+} A(x+\eta)$. The above equations involve the interaction vertex $\Gamma(1,2;3)$, the fully-interacting one-body Green's function $G(1,2)$, and the reference Green's function $G^0(1,2)$, the self-energy $\Sigma(1,2) = \Sigma_H(1,2) + \Sigma_{xc}(1,2)$, formally split into the Hartree self-energy $\Sigma_H$ and the exchange-correlation self-energy $\Sigma_{xc}$, the polarization function $P(1,2)$, the bare Coulomb interaction $v(1,2) = \delta(t_1-t_2)\frac{1}{|\vec{r}_1-\vec{r}_2|}$, and the screened Coulomb interaction $W(1,2)$.

When writing these magnitude in orbital basis, only $G$ and $\Sigma$ remain two-index quantities, while the rest are defined by four orbital indices and up to three time indices. The number of indices corresponds to the number of external legs for the corresponding Feynman diagram. In the orbital basis, Hedin's equations read

$$\begin{aligned}\Gamma^{l\sigma_l;\; j\sigma_j}_{i\sigma_i;\; k\sigma_k}\left(t_i,t_j;t_j^+,t_k\right) = {}& \delta^{\sigma_i,\sigma_l}_{i,l}\delta^{\sigma_j,\sigma_k}_{j,k}\delta(t_i-t_j^+)\delta(t_k-t_j) \\ & + \frac{\delta\Sigma^{xc}_{i\sigma_i;\; k\sigma_k}(t_i;t_k)}{\delta G_{m\sigma_m;\; n\sigma_n}\left(\bar{t}_m^+;\bar{t}_m\right)} G_{m\sigma_m;\; x\sigma_x}\left(\bar{t}_m^+;\bar{t}_x\right)\Gamma^{l\sigma_l;\; j\sigma_j}_{x\sigma_x;\; y\sigma_y}\left(\bar{t}_x,t_j;t_j^+,\bar{t}_y\right)G_{y\sigma_y;\; n\sigma_n}\left(\bar{t}_y;\bar{t}_m\right),\end{aligned} \tag{12}$$

$$P^{l\sigma_l;\; j\sigma_j}_{i\sigma_i;\; k\sigma_k}\left(t_i,t_j^+;t_j,t_k\right) = -iG_{i\sigma_i;\; m\sigma_m}(t_i;\bar{t}_m)\Gamma^{l\sigma_l;\; j\sigma_j}_{m\sigma_m;\; n\sigma_n}\left(\bar{t}_m,t_j;t_j^+,\bar{t}_n\right)G_{n\sigma_n;\; k\sigma_k}(\bar{t}_n;t_k), \tag{13}$$

$$W^{l\sigma_l;\; j\sigma_j}_{i\sigma_i;\; k\sigma_k}\left(t_i,t_j;t_i^+,t_j^+\right) = v^{l\sigma_l;\; j\sigma_j}_{i\sigma_i;\; k\sigma_k}\delta(t_i-t_j) + v^{k\sigma_k;\; t\sigma_t}_{j\sigma_j;\; u\sigma_u}P^{x\sigma_x;\; y\sigma_y}_{u\sigma_u;\; t\sigma_t}\left(t_j,\bar{t}_x^+;\bar{t}_x,t_j^+\right)W^{l\sigma_l;\; x\sigma_x}_{i\sigma_i;\; y\sigma_y}\left(t_i,\bar{t}_x;t_i^+,\bar{t}_x^+\right), \tag{14}$$

$$\Sigma^{xc}_{i\sigma_i;\; j\sigma_j}(t_i;t_j) = iW^{s\sigma_s;\; m\sigma_m}_{i\sigma_i;\; n\sigma_n}\left(t_i^+,\bar{t}_n^+;t_i^{++},\bar{t}_n\right)G_{s\sigma_s;\; t\sigma_t}(t_i;\bar{t}_t)\Gamma^{m\sigma_m;\; n\sigma_n}_{t\sigma_t;\; j\sigma_j}\left(\bar{t}_t,\bar{t}_n;\bar{t}_n^+,t_j\right), \tag{15}$$

$$G_{i\sigma_i;\; j\sigma_j}(t_i;t_j) = G^0_{i\sigma_i;\; j\sigma_j}(t_i;t_j) + G^0_{i\sigma_i;\; a\sigma_a}(t_i;\bar{t}_a)\Sigma_{a\sigma_a;\; b\sigma_b}(\bar{t}_a;\bar{t}_b)G_{b\sigma_b;\; j\sigma_j}(\bar{t}_b;t_j). \tag{16}$$

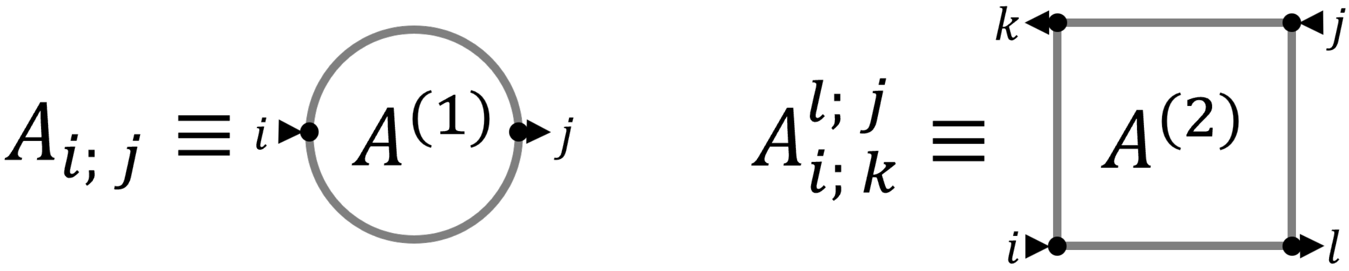


FIG. 2. Diagrammatic and formula representations for two- and four-index quantities.

In the above equations, summation over repeated orbital and spin indices is assumed, and barred time arguments are integrated over. Two-index quantities (such as the Green's function and self-energy) transform between real space and orbital bases as

$$A_{i\sigma_i;\ j\sigma_j}(t_1;t_2) = \int \mathrm{d}\vec{r}_1 \mathrm{d}\vec{r}_2\ \phi_i^*(\vec{r}_1) A^{(1)}(1,2)\phi_j(\vec{r}_2), \tag{17}$$

while four index quantities (the interaction potentials, polarization function and interaction vertex) transform as

$$A^{l\sigma_l;\ j\sigma_j}_{i\sigma_i;\ k\sigma_k}(t_1,t_2;t_3,t_4) = \int \mathrm{d}\vec{r}_1 \mathrm{d}\vec{r}_2\ \phi_i^*(\vec{r}_1)\phi_l(\vec{r}_1) A^{(2)}(\vec{r}_1,\vec{r}_2;t_1,t_2,t_3,t_4)\phi_j^*(\vec{r}_2)\phi_k(\vec{r}_2), \tag{18}$$

where we allow the four-index quantity $A^{(2)}(1,2)$ to formally depend of up to four time indices. The internal structure of the particular quantities decreases the number of time variables, e.g. $v$ being time independent and $W$ depending only of a single time difference. A diagrammatic representation of two- and four-index quantities is given in Fig. 2.

In principle, Eq. (12)- (16) can be derived from the real space counterparts by using the relations in Eq. (17) and (18) and the completeness relations for the orbital and real space bases. However, this calls for tedious calculations with careful index tracking, with little physical insight. Instead, we find it is more instructive to derive Hedin's equations in orbital space directly, from the equation of motion of the one body Green's function. We turn hence now our attention to this derivation, following closely the real-part counterpart which can be found e.g. in Chap. 10 and 11 in Ref. [2].

### A. Derivation of Hedin's equations in orbital space

We will consider a number and spin conserving Fermionic Hamiltonian written in terms of one- and two-body terms as

$$H = h_{p,q} c^\dagger_{p,\sigma} c_{q,\sigma} + \frac{1}{2} v^{s\sigma;\ q\sigma'}_{p\sigma;\ r\sigma'} c^\dagger_{p,\sigma} c^\dagger_{q,\sigma'} c_{r,\sigma'} c_{s,\sigma}, \tag{19}$$

where we keep the implied sum over repeated indices. Note how both the one-body Hamiltonian $h$ and the bare Coulomb interaction$v$ preserve the total spin and spin projection. To simplify the notation, we will further introduce the following four-spin expression for the bare Coulomb interaction$v$

$$v^{l\sigma_l;\ j\sigma_j}_{i\sigma_i;\ k\sigma_k} \equiv v^{l\sigma_i;\ j\sigma_j}_{i\sigma_i;\ k\sigma_j}\ \delta^{\sigma_i,\sigma_l}\delta^{\sigma_j,\sigma_k}. \tag{20}$$

We start the derivation of Hedin's equations with the definition of the one-body Green's function, which follows

$$G_{i\sigma_i;\ j\sigma_j}(t_i;t_j) = -i\langle \mathcal{T}\left\{ c_{i\sigma_i}(t_i) c^\dagger_{j\sigma_j}(t_j)\right\}\rangle = -i\theta(t_i-t_j)\langle c_{i\sigma_i}(t_i) c^\dagger_{j\sigma_j}(t_j)\rangle + i\theta(t_i-t_j)\langle c^\dagger_{j\sigma_j}(t_j) c_{i\sigma_i}(t_i)\rangle, \tag{21}$$

where $\mathcal{T}$ represents the time-ordering operator, $\langle\cdot\rangle$ is some appropriate average, and $c_{a\sigma_a}(t_a) = e^{iHt_a} c_{a\sigma_a} e^{-iHt_a}$ is the Heisenberg representation of operator $c_{a\sigma_a}$. It is not hard to show that the equation of motion for the annihilation operators obeys

$$i\frac{\partial}{\partial t_m} c_{m\sigma_m}(t_m) = h_{m,p} c_{p\sigma_m}(t_m) + v^{s\sigma_s;\ q\sigma_q}_{m\sigma_m;\ r\sigma_r} c^\dagger_{q\sigma_q}(t_m) c_{r\sigma_r}(t_m) c_{s\sigma_s}(t_m). \tag{22}$$

With this, we can write the equation of motion for the one-body Green's function $G$ as

$$\left(i\delta^{\sigma_p,\sigma_p}_{p,i}\frac{\partial}{\partial t_i} - h_{i,p}\delta^{\sigma_i,\sigma_p}\right) G_{p\sigma_p;\ j\sigma_j}(t_i;t_j) + i\, v^{s\sigma_s;\ q\sigma_q}_{i\sigma_i;\ r\sigma_r} \Lambda^{j\sigma_j;\ r\sigma_r}_{s\sigma_s;\ q\sigma_q}\left(t_i, t_i^+; t_j, t_i^{++}\right) = \delta_{i,j}\delta_{\sigma_i,\sigma_j}\delta(t_i - t_j), \tag{23}$$

where we have introduced the two-body Green's function $\Lambda^{l\sigma_l;\ j\sigma_j}_{i\sigma_i;\ k\sigma_k}(t_i, t_j; t_l, t_k)$ as

$$\Lambda^{l\sigma_l;\ j\sigma_j}_{i\sigma_i;\ k\sigma_k}(t_i, t_j; t_l, t_k) = -\langle \mathcal{T}\left\{c_{i\sigma_i}(t_i) c_{j\sigma_j}(t_j) c^\dagger_{k\sigma_k}(t_k) c^\dagger_{l\sigma_l}(t_l)\right\}\rangle, \tag{24}$$

Now, we can solve Eq. (23) for the one-body Green's function $G$ by introducing the non-interacting Green's function $G^0$ in the usual way as

$$\left(i\delta^{\sigma_p,\sigma_p}_{p,i}\frac{\partial}{\partial t_i} - h_{i,p}\delta^{\sigma_i,\sigma_p}\right) G^0_{p\sigma_p;\ j\sigma_j}(t_i;t_j) = \delta_{i,j}\delta_{\sigma_i,\sigma_j}\delta(t_i - t_j), \tag{25}$$

such that we can write

$$G_{i\sigma_i;\ j\sigma_j}(t_i;t_j) = G^0_{i\sigma_i;\ j\sigma_j}(t_i;t_j) - iG^0_{i\sigma_i;\ q\sigma_q}(t_i;\bar{t}_q)\, v^{s\sigma_s;\ p\sigma_p}_{q\sigma_q;\ r\sigma_r} \Lambda^{j\sigma_j;\ r\sigma_r}_{s\sigma_s;\ p\sigma_p}\left(\bar{t}_q, \bar{t}_q^+; t_j, \bar{t}_q^{++}\right), \tag{26}$$

This equation allows the evaluation of $G$ in terms of the non-interacting Green's function $G^0$, which can be calculated easily from Eq. (25), and the two-body Green's function $\Lambda$. To obtain some degree of closeness, we turn now to expressing the latter as a functional derivative of $G$ with respect to an external, probing field. This can be accomplished within Schwinger's functional derivative formalism, common in field theory.

Indeed, we can define the grand canonical potential $\Omega$ for Hamiltonian $H$ under the presence of an external, one-body field $u$ as

$$\Omega[u] = -\frac{1}{\beta}\ln Z[u] = -\frac{1}{\beta}\ln \mathrm{Tr}\left[e^{-\beta(H-\mu N)}\mathcal{T} e^{iu_{p\sigma_p;\ q\sigma_q}(\bar{t}_p;\bar{t}_q) c^\dagger_{p\sigma_p}(\bar{t}_p) c_{q\sigma_q}(\bar{t}_q)}\right], \tag{27}$$

where we have introduced the chemical potential $\mu$, the inverse temperature $\beta$, the total number operator $N$, and the partition function under the presence of an external potential $Z[u]$. It is easy to verify that we can write the fully interacting one-body Green's function as a functional derivative of $G$, namely

$$G_{p\sigma_p;\ s\sigma_s}(t_p;t_s) = \beta\left.\frac{\delta\Omega[u]}{\delta u_{s\sigma_s;\ p\sigma_p}(t_s;t_p)}\right|_{u=0}. \tag{28}$$

Moreover, we can relate the two-body Green's function $\Lambda$ to a second order functional derivative of $\Omega$, hence to a functional derivative of $G$, by introducing the auxiliary correlation function $L$

$$\begin{aligned} L^{s\sigma_s;\ q\sigma_q}_{p\sigma_p;\ r\sigma_r}(t_p, t_q; t_s, t_r) &\equiv -\Lambda^{s\sigma_s;\ q\sigma_q}_{p\sigma_p;\ r\sigma_r}(t_p, t_q; t_s, t_r) + G_{q\sigma_q;\ r\sigma_r}(t_q;t_r)\, G_{p\sigma_p;\ s\sigma_s}(t_p;t_s) \\ &= \beta\left.\frac{\delta}{\delta u_{r\sigma_r;\ q\sigma_q}(t_r;t_q)}\left[\frac{\delta\Omega[u]}{\delta u_{s\sigma_s;\ p\sigma_p}(t_s;t_p)}\right]\right|_{u=0} = \left.\frac{\delta G_{p\sigma_p;\ s\sigma_s}(t_p;t_s)}{\delta u_{r\sigma_r;\ q\sigma_q}(t_r;t_q)}\right|_{u=0}. \end{aligned} \tag{29}$$

From it's definition, we see that $L$ encodes the non-trivial (fundamentally two-body) correlations encoded in the two-body Green's function $\Lambda$. With this relation, we can rewrite Eq. (26) as

$$\begin{aligned}G_{i\sigma_i;\ j\sigma_j}\left(t_i;t_j\right) &= G^{(0)}_{i\sigma_i;\ j\sigma_j}\left(t_i;t_j\right)\\ &+ G^{0}_{i\sigma_i;\ q\sigma_q}\left(t_i;\bar{t}_q\right)\left(\left[-iv^{s\sigma_s;\ p\sigma_p}_{q\sigma_q;\ r\sigma_r}G_{r\sigma_r;\ p\sigma_p}\left(\bar{t}_q^{+};\bar{t}_q^{++}\right)\right]G_{s\sigma_s;\ j\sigma_j}\left(\bar{t}_q;t_j\right) + iv^{s\sigma_s;\ p\sigma_p}_{q\sigma_q;\ r\sigma_r}L^{j\sigma_j;\ r\sigma_r}_{s\sigma_s;\ p\sigma_p}\left(\bar{t}_q,t_j;\bar{t}_q^{+},\bar{t}_q^{++}\right)\right),\\ &= G^{(0)}_{i\sigma_i;\ j\sigma_j}\left(t_i;t_j\right) + G^{0}_{i\sigma_i;\ q\sigma_q}\left(t_i;\bar{t}_q\right)\left(v^{H}_{q\sigma_q;\ s\sigma_s}\left(\bar{t}_q^{+};\bar{t}_s\right)G_{s\sigma_s;\ j\sigma_j}\left(\bar{t}_q;t_j\right) + iv^{s\sigma_s;\ p\sigma_p}_{q\sigma_q;\ r\sigma_r}\left.\frac{\delta G_{s\sigma_s;\ j\sigma_j}\left(\bar{t}_q;t_j\right)}{\delta u_{p\sigma_p;\ r\sigma_r}\left(\bar{t}_q^{++};\bar{t}_q^{+}\right)}\right|_{u=0}\right).\end{aligned} \tag{30}$$

where in the second line we have identified the Hartree-potential

$$v^{H}_{i\sigma_i;\ j\sigma_j}\left(t_i;t_j\right) = -iv^{j\sigma_j;\ p\sigma_p}_{i\sigma_i;\ q\sigma_q}G_{q\sigma_q;\ p\sigma_p}\left(t_i;t_i^{+}\right)\delta(t_i-t_j), \tag{31}$$

which is instantaneous in time, but while local in real space, potentially non-local in orbital space. By virtue of the spin structure of $v$ (c.f. Eq. (20)), it is however "local" in spin, i.e. only same spin electrons interact through the Hartree potential. Eq. (30) can be brought into the usual Dyson form of Eq. (16) by making, after one minor manipulation[7], the following identification for the self-energy $\Sigma$

$$\begin{aligned}\Sigma_{i\sigma_i;\ j\sigma_j}\left(t_i;t_j\right) &= v^{H}_{i\sigma_i;\ j\sigma_j}\left(t_i;t_j\right) - iv^{s\sigma_s;\ p\sigma_p}_{i\sigma_i;\ r\sigma_r}G_{s\sigma_s;\ t\sigma_t}\left(t_i;\bar{t}_t\right)\left.\frac{\delta G^{-1}_{t\sigma_t;\ j\sigma_j}\left(\bar{t}_t;t_j\right)}{\delta u_{p\sigma_p;\ r\sigma_r}\left(t_i^{++};t_i^{+}\right)}\right|_{u=0},\\ &= \Sigma^{H}_{i\sigma_i;\ j\sigma_j}\left(t_i;t_j\right) + \Sigma^{xc}_{i\sigma_i;\ j\sigma_j}\left(t_i;t_j\right),\end{aligned} \tag{32}$$

where in the last line we define the Hartree and exchange-correlation component of the self-energy. While Eq. (32) and the Dyson Eq. (16) already present a closed system of equations for $G$ and $\Sigma$, they involve the external, artificial, probing field $u$. We note that this field depends on two orbitals (it corresponds to a two-legged diagram), but crucially it only enters the self-energy equation as a one-time quantity $u(t) \equiv u(t^{+},t)$. Keeping this time structure in the back of our minds will be important for later.

The main idea in Hedin's equations is rewriting the system of equations given by Eq. (32) and (16) as a more involved but crucially "self-contained" one, i.e. one which avoids any reference to external quantities. With this goal in mind, let us define the total classical potential $v^{cl}$ as the sum of the external probing potential $u$ and the Hartree-potential $v^{H}$

$$v^{cl}_{i\sigma_i;\ j\sigma_j}\left(t_i;t_j\right) = u_{i\sigma_i;\ j\sigma_j}\left(t_i;t_j\right) + v^{H}_{i\sigma_i;\ j\sigma_j}\left(t_i;t_j\right). \tag{33}$$

Given that $v^{cl}$ represents to total electrostatic potential present in the system, with or without external probing potential, a promising strategy would be to rewrite the functional derivatives with respect to $u$ into functional derivatives with respect to $v^{cl}$. To do this, we will need the "Jacobian" $\delta v^{cl}/\delta u$ [8], which is of course nothing but the inverse dielectric function $\epsilon^{-1}$, i.e. the linear term in the change of electrostatic potential in the system as a response to an external field. With some algebra, we can write this in terms of the Green's function as

$$\begin{aligned}\epsilon^{-1}{}^{m\sigma_m;\ n\sigma_n}_{i\sigma_i;\ j\sigma_j}\left(t_i,t_n;t_m,t_j\right) &= \frac{\delta v^{cl}_{i\sigma_i;\ j\sigma_j}\left(t_i;t_j\right)}{\delta u_{m\sigma_m;\ n\sigma_n}\left(t_m;t_n\right)}\\ &= \delta^{\sigma_i,\sigma_m}_{i,m}\delta^{\sigma_n,\sigma_j}_{n,j}\delta(t_i-t_m)\delta(t_j-t_n) - iv^{j\sigma_j;\ p\sigma_p}_{i\sigma_i;\ q\sigma_q}\frac{\delta G_{q\sigma_q;\ p\sigma_p}\left(t_i;t_i^{++}\right)}{\delta u_{m\sigma_m;\ n\sigma_n}\left(t_m;t_n\right)}\delta(t_i-t_j).\end{aligned} \tag{34}$$

Note that for simplicity, here and henceforth we drop the explicit indication of the limit $u=0$ in the functional derivatives. We can now change the functional derivative with respect to $u$ in Eq. (32) into a product of $\epsilon^{-1}$ and a functional derivative with respect to the total potential. Indeed, by using the chain rule, we find

$$\begin{aligned}
\Sigma^{xc}_{i\sigma_i;\; j\sigma_j}\left(t_i;t_j\right) &= -iv^{s\sigma_s;\; p\sigma_p}_{i\sigma_i;\; r\sigma_r} G_{s\sigma_s;\; t\sigma_t}\left(t_i;\bar{t}_t\right) \frac{\delta G^{-1}_{t\sigma_t;\; j\sigma_j}\left(\bar{t}_t;t_j\right)}{\delta u_{p\sigma_p;\; r\sigma_r}\left(t_i^{++};t_i^{+}\right)}, \\
&= -iv^{s\sigma_s;\; p\sigma_p}_{i\sigma_i;\; r\sigma_r} G_{s\sigma_s;\; t\sigma_t}\left(t_i;\bar{t}_t\right) \frac{\delta G^{-1}_{t\sigma_t;\; j\sigma_j}\left(\bar{t}_t;t_j\right)}{\delta v^{cl}_{m\sigma_m;\; n\sigma_n}\left(\bar{t}_m^{++};\bar{t}_m^{+}\right)} \frac{\delta v^{cl}_{m\sigma_m;\; n\sigma_n}\left(\bar{t}_m^{++};\bar{t}_m^{+}\right)}{\delta u_{p\sigma_p;\; r\sigma_r}\left(t_i^{++};t_i^{+}\right)}, \\
&= -iv^{s\sigma_s;\; p\sigma_p}_{i\sigma_i;\; r\sigma_r} \epsilon^{-1}{}^{\;p\sigma_p;\; r\sigma_r}_{\;m\sigma_m;\; n\sigma_n}\left(\bar{t}_m^{++},t_i^{+};t_i^{++},\bar{t}_m^{+}\right) G_{s\sigma_s;\; t\sigma_t}\left(t_i;\bar{t}_t\right) \Gamma^{m\sigma_m;\; n\sigma_n}_{t\sigma_t;\; j\sigma_j}\left(\bar{t}_t,\bar{t}_m^{+};\bar{t}_m^{++},t_j\right) \\
&= -iW^{s\sigma_s;\; m\sigma_m}_{i\sigma_i;\; n\sigma_n}\left(t_i^{+},t_m^{++};\bar{t}_i^{++},\bar{t}_m^{+}\right) G_{s\sigma_s;\; t\sigma_t}\left(t_i;\bar{t}_t\right) \Gamma^{m\sigma_m;\; n\sigma_n}_{t\sigma_t;\; j\sigma_j}\left(\bar{t}_t,\bar{t}_m^{+};\bar{t}_m^{++},t_j\right).
\end{aligned} \tag{35}$$

After applying the chain rule in the second line, in the third line we use Eq. (34) and define the interaction vertex $\Gamma$ as

$$\Gamma^{m\sigma_m;\; n\sigma_n}_{t\sigma_t;\; j\sigma_j}\left(t_t,t_m^{+};t_m^{++},t_j\right) = -\frac{\delta G^{-1}_{t\sigma_t;\; j\sigma_j}\left(t_t;t_j\right)}{\delta v^{cl}_{m\sigma_m;\; n\sigma_n}\left(t_m^{++};t_m^{+}\right)}, \tag{36}$$

and finally in the fourth line in Eq. (35) we recognize that the screened interaction $W$ is obtained from the bare interaction $v$ by contraction with $\epsilon^{-1}$ as

$$W^{s\sigma_s;\; m\sigma_m}_{i\sigma_i;\; n\sigma_n}\left(t_i,t_m^{+};t_i^{+},t_m\right) = \epsilon^{-1}{}^{\;p\sigma_p;\; r\sigma_r}_{\;m\sigma_m;\; n\sigma_n}\left(t_m^{+},t_i;t_i^{+},t_m\right) v^{s\sigma_s;\; p\sigma_p}_{i\sigma_i;\; r\sigma_r}. \tag{37}$$

Note how the time structure of $u(t) \equiv u(t^{+},t)$ propagates through the equations, such that only the expected two-time form of the screened interaction $W$ appears. Similarly, the interaction vertex $\Gamma$ depends on four orbitals, but its component entering the equations depends formally only on three times.

We note that we have already derived two of the five Hedin's equations: the Dyson equation (c.f. Eq. (16) and (30)/ (32)) and the self-energy equation in terms of the interaction vertex and screened Coulomb interaction (c.f. Eq. (15) and (35)). To advance, we need to express the inverse dielectric function $\epsilon^{-1}$ in terms of the interaction vertex, and we need to find a closed expression for the latter avoiding the inclusion of the classical potential.

Le us first turn our attention to $\epsilon^{-1}$. The offending term in Eq. (34) is the functional derivative of $G$ with respect to $u$. We can deal with is as we have done in Eq. (35): using the chain rule. Thus, we find

$$\begin{aligned}
-i\frac{\delta G_{i\sigma_i;\; j\sigma_j}\left(t_i;t_j\right)}{\delta u_{m\sigma_m;\; n\sigma_n}\left(t_m;t_n\right)} &= -i\frac{\delta G_{i\sigma_i;\; j\sigma_j}\left(t_i;t_j\right)}{\delta v^{cl}_{p\sigma_p;\; q\sigma_q}\left(\bar{t}_p;\bar{t}_q\right)} \frac{\delta v^{cl}_{p\sigma_p;\; q\sigma_q}\left(\bar{t}_p;\bar{t}_q\right)}{\delta u_{m\sigma_m;\; n\sigma_n}\left(t_m;t_n\right)}, \\
&= P^{p\sigma_p;\; q\sigma_q}_{i\sigma_i;\; j\sigma_j}\left(t_i,\bar{t}_q;\bar{t}_p,t_j\right) \epsilon^{-1}{}^{\;m\sigma_m;\; n\sigma_n}_{\;p\sigma_p;\; q\sigma_q}\left(\bar{t}_p,t_n;t_m,\bar{t}_q\right),
\end{aligned} \tag{38}$$

where we have identified $\epsilon^{-1}$ in the second line, as well as defined the polarization function

$$P^{l\sigma_l;\; j\sigma_j}_{i\sigma_i;\; k\sigma_k}\left(t_i,t_j;t_l,t_k\right) = -i\frac{\delta G_{i\sigma_i;\; k\sigma_k}\left(t_i;t_k\right)}{\delta v^{cl}_{l\sigma_l;\; j\sigma_j}\left(t_l;t_j\right)}. \tag{39}$$

And we can rewrite this in terms of the interaction vertex following

$$\begin{aligned}
P^{l\sigma_l;\; j\sigma_j}_{i\sigma_i;\; k\sigma_k}\left(t_i,t_j;t_l,t_k\right) &= -i\frac{\delta G_{i\sigma_i;\; k\sigma_k}\left(t_i;t_k\right)}{\delta v^{cl}_{l\sigma_l;\; j\sigma_j}\left(t_l;t_j\right)}, \\
&= iG_{i\sigma_i;\; m\sigma_m}\left(t_i;\bar{t}_m\right) \frac{\delta G^{-1}_{m\sigma_m;\; n\sigma_n}\left(\bar{t}_m;\bar{t}_n\right)}{\delta v^{cl}_{l\sigma_l;\; j\sigma_j}\left(t_l;t_j\right)} G_{n\sigma_n;\; k\sigma_k}\left(\bar{t}_n;t_k\right), \\
&= iG_{i\sigma_i;\; m\sigma_m}\left(t_i;\bar{t}_m\right) \Gamma^{l\sigma_l;\; j\sigma_j}_{m\sigma_m;\; n\sigma_n}\left(\bar{t}_m,t_l;t_j,\bar{t}_n\right) G_{n\sigma_n;\; k\sigma_k}\left(\bar{t}_n;t_k\right),
\end{aligned} \tag{40}$$

which reduces to Eq. (13) once the proper limits are applied on the time arguments. With this result, we can rewrite the screened interaction without explicitly invoking the dielectric function, by turning Eq. (37) into a “recursive” (i.e. Dyson-like) equation

$$
\begin{aligned}
W^{s\sigma_s;\; m\sigma_m}_{i\sigma_i;\; n\sigma_n}\left(t_i, t_m^+; t_i^+, t_m\right) &= \epsilon^{-1}\,{}^{p\sigma_p;\; r\sigma_r}_{m\sigma_m;\; n\sigma_n}\left(t_m^+, t_i; t_i^+, t_m\right) v^{s\sigma_s;\; p\sigma_p}_{i\sigma_i;\; r\sigma_r},\\
&= v^{s\sigma_s;\; m\sigma_m}_{i\sigma_i;\; n\sigma_n}\delta(t_i - t_m) + v^{s\sigma_s;\; p\sigma_p}_{i\sigma_i;\; r\sigma_r} v^{n\sigma_n;\; t\sigma_t}_{m\sigma_m;\; u\sigma_u} P^{x\sigma_x;\; y\sigma_y}_{u\sigma_u;\; t\sigma_t}\left(t_m, \bar{t}_x^+; \bar{t}_x, t_m^+\right) \epsilon^{-1}\,{}^{p\sigma_p;\; r\sigma_r}_{x\sigma_x;\; y\sigma_y}\left(\bar{t}_x^+, t_i; t_i^+, \bar{t}_x\right),\\
&= v^{s\sigma_s;\; m\sigma_m}_{i\sigma_i;\; n\sigma_n}\delta(t_i - t_m) + v^{n\sigma_n;\; t\sigma_t}_{m\sigma_m;\; u\sigma_u} P^{x\sigma_x;\; y\sigma_y}_{u\sigma_u;\; t\sigma_t}\left(t_m, \bar{t}_x^+; \bar{t}_x, t_m^+\right) W^{s\sigma_s;\; x\sigma_x}_{i\sigma_i;\; y\sigma_y}\left(t_i, \bar{t}_x^+; t_i^+, \bar{t}_x\right).
\end{aligned}
\tag{41}
$$

This corresponds to Eq. (14).

Finally, we can also rid the definition of the interaction vertex $\Gamma$ in Eq. (36) from any explicit reference to the total potential $v^{cl}$ by making it into a Dyson-like equation

$$
\begin{aligned}
\Gamma^{l\sigma_l;\; j\sigma_j}_{i\sigma_i;\; k\sigma_k}\left(t_i, t_j; t_j^+, t_k\right) &= -\frac{\delta G^{-1}_{i\sigma_i;\; k\sigma_k}\left(t_i; t_k\right)}{\delta v^{cl}_{l\sigma_l;\; j\sigma_j}\left(t_j^+; t_j\right)},\\
&= -\frac{\delta}{\delta v^{cl}_{l\sigma_l;\; j\sigma_j}\left(t_j^+; t_j\right)}\left[\delta^{\sigma_i,\sigma_k}_{i,k}\delta(t_i - t_k) - v^{cl}_{i\sigma_i;\; k\sigma_k}\left(t_i; t_k\right) - \Sigma^{xc}_{i\sigma_i;\; k\sigma_k}\left(t_i; t_k\right)\right],\\
&= \delta^{\sigma_i,\sigma_l}_{i,l}\delta^{\sigma_j,\sigma_k}_{j,k} + \frac{\delta \Sigma^{xc}_{i\sigma_i;\; k\sigma_k}\left(t_i; t_k\right)}{\delta G_{m\sigma_m;\; n\sigma_n}\left(\bar{t}_m; \bar{t}_n\right)} \frac{\delta G_{m\sigma_m;\; n\sigma_n}\left(\bar{t}_m; \bar{t}_n\right)}{\delta v^{cl}_{l\sigma_l;\; j\sigma_j}\left(t_j^+; t_j\right)},\\
&= \delta^{\sigma_i,\sigma_l}_{i,l}\delta^{\sigma_j,\sigma_k}_{j,k} - \frac{\delta \Sigma^{xc}_{i\sigma_i;\; k\sigma_k}\left(t_i; t_k\right)}{\delta G_{m\sigma_m;\; n\sigma_n}\left(\bar{t}_m; \bar{t}_n\right)} G_{m\sigma_m;\; x\sigma_x}\left(\bar{t}_m; \bar{t}_x\right) \frac{\delta G^{-1}_{x\sigma_x;\; y\sigma_y}\left(\bar{t}_x; \bar{t}_y\right)}{\delta v^{cl}_{l\sigma_l;\; j\sigma_j}\left(t_j^+; t_j\right)} G_{y\sigma_y;\; n\sigma_n}\left(\bar{t}_y; \bar{t}_n\right),\\
&= \delta^{\sigma_i,\sigma_l}_{i,l}\delta^{\sigma_j,\sigma_k}_{j,k} + \frac{\delta \Sigma^{xc}_{i\sigma_i;\; k\sigma_k}\left(t_i; t_k\right)}{\delta G_{m\sigma_m;\; n\sigma_n}\left(\bar{t}_m; \bar{t}_n\right)} G_{m\sigma_m;\; x\sigma_x}\left(\bar{t}_m; \bar{t}_x\right) \Gamma^{l\sigma_l;\; j\sigma_j}_{x\sigma_x;\; y\sigma_y}\left(\bar{t}_x, t_j; t_j^+, \bar{t}_y\right) G_{y\sigma_y;\; n\sigma_n}\left(\bar{t}_y; \bar{t}_n\right),
\end{aligned}
\tag{42}
$$

which recovers Eq. (12).

In this way, we have derived Hedin's equations in orbital space. In the next sections, we derive from these core equations the approximations employed in the main paper, which correspond to different expansions for the functional derivative $\delta\Sigma^{xc}/\delta G$ in the $\Gamma$ equation.

## III. PERTURBATIVE APPROXIMATIONS IN THE MAIN PAPER

In this section we give the equations defining the different perturbative approximations employed in the main paper. This correspond to adapting Hedin's equations in Eq. (12)- (16) by introducing different approximations to the functional derivative $\delta\Sigma^{xc}/\delta G$, which we successively refine in terms of the four interaction kernels $\mathcal{K}$ introduced in the paper. These arise in the functional derivative by substituting the formal expression for $\Sigma^{xc}$ in terms of $G$, $W$ and $\Gamma$. These are, explicitly

$$
\begin{aligned}
\frac{\delta \Sigma^{xc}_{i\sigma_i;\; k\sigma_k}\left(t_i; t_k\right)}{\delta G_{m\sigma_m;\; n\sigma_n}\left(t_m; t_n\right)} &= 0\\
&\quad + i\frac{\delta G_{s\sigma_s;\; t\sigma_t}\left(t_i; \bar{t}_t\right)}{\delta G_{m\sigma_m;\; n\sigma_n}\left(t_m; t_n\right)} W^{s\sigma_s;\; x\sigma_x}_{i\sigma_i;\; y\sigma_y}\left(t_i^+, \bar{t}_x^+; t_i^{++}, \bar{t}_x\right) \Gamma^{x\sigma_x;\; y\sigma_y}_{t\sigma_t;\; j\sigma_j}\left(\bar{t}_t, \bar{t}_x^+; \bar{t}_x, t_j\right)\\
&\quad + iG_{s\sigma_s;\; t\sigma_t}\left(t_i; \bar{t}_t\right) \frac{\delta W^{s\sigma_s;\; x\sigma_x}_{i\sigma_i;\; y\sigma_y}\left(t_i^+, \bar{t}_x^+; t_i^{++}, \bar{t}_x\right)}{\delta G_{m\sigma_m;\; n\sigma_n}\left(t_m; t_n\right)} \Gamma^{x\sigma_x;\; y\sigma_y}_{t\sigma_t;\; j\sigma_j}\left(\bar{t}_t, \bar{t}_x^+; \bar{t}_x, t_j\right)\\
&\quad + iG_{s\sigma_s;\; t\sigma_t}\left(t_i; \bar{t}_t\right) W^{s\sigma_s;\; x\sigma_x}_{i\sigma_i;\; y\sigma_y}\left(t_i^+, \bar{t}_x^+; t_i^{++}, \bar{t}_x\right) \frac{\delta \Gamma^{x\sigma_x;\; y\sigma_y}_{t\sigma_t;\; j\sigma_j}\left(\bar{t}_t, \bar{t}_x^+; \bar{t}_x, t_j\right)}{\delta G_{m\sigma_m;\; n\sigma_n}\left(t_m; t_n\right)},\\
&= \mathcal{K}_0\,{}^{m\sigma_m;\; n\sigma_n}_{i\sigma_i;\; k\sigma_k}\left(t_i, t_n; t_m, t_k\right) + \mathcal{K}_G\,{}^{m\sigma_m;\; n\sigma_n}_{i\sigma_i;\; k\sigma_k}\left(t_i, t_n; t_m, t_k\right)\\
&\quad + \mathcal{K}_W\,{}^{m\sigma_m;\; n\sigma_n}_{i\sigma_i;\; k\sigma_k}\left(t_i, t_n; t_m, t_k\right) + \mathcal{K}_\Gamma\,{}^{m\sigma_m;\; n\sigma_n}_{i\sigma_i;\; k\sigma_k}\left(t_i, t_n; t_m, t_k\right).
\end{aligned}
\tag{43}
$$

In the following subsections, we will motivate the different approximations, providing with the exact expressions used to implement them, and sketching the derivation of said expressions.

A general note before turning to the particular approximations: We have given Hedin's equations in Eq. (12)- (16) in terms of real time. However, as a consequence, several of them involve time integrals, which can be cumbersome

to implement numerically. Instead, it is often convenient to transform the equations into frequency space, by Fourier transform. In many cases, invoking the time translational symmetry in equilibrium problems and the convolution theorem, we can turn the integrals in real time into products in frequency space. In particular, we can exploit that in equilibrium we necessarily have

$$\begin{aligned}
G_{i\sigma_i;\ j\sigma_j}\left(t_i;t_j\right) &\equiv G_{i\sigma_i;\ j\sigma_j}\left(t_i-t_j\right),\\
\Sigma_{i\sigma_i;\ j\sigma_j}\left(t_i;t_j\right) &\equiv \Sigma_{i\sigma_i;\ j\sigma_j}\left(t_i-t_j\right),\\
W^{l\sigma_l;\ j\sigma_j}_{i\sigma_i;\ k\sigma_k}\left(t_i,t_j;t_i^+,t_j^+\right) &\equiv W^{l\sigma_l;\ j\sigma_j}_{i\sigma_i;\ k\sigma_k}\left(t_i-t_j\right),\\
P^{l\sigma_l;\ j\sigma_j}_{i\sigma_i;\ k\sigma_k}\left(t_i,t_j^+;t_j,t_i\right) &\equiv P^{l\sigma_l;\ j\sigma_j}_{i\sigma_i;\ k\sigma_k}\left(t_i-t_j;t_j-t_i\right) \equiv \tilde{P}^{l\sigma_l;\ j\sigma_j}_{i\sigma_i;\ k\sigma_k}\left(t_j-t_i\right).
\end{aligned} \tag{44}$$

Where in the third equation we have used the fact that, in equilibrium, the screened Coulomb interaction can only depend on one time, namely the time difference between the emission and absorption of the dressed photon. Hence, we can for instance rewrite the equations for $G$ and $W$ (i.e. Eq. (16) and (14)) in frequency space as

$$\begin{aligned}
G_{i\sigma_i;\ j\sigma_j}\left(\omega\right) &= G^0_{i\sigma_i;\ j\sigma_j}\left(\omega\right) + G^0_{i\sigma_i;\ a\sigma_a}\left(\omega\right)\Sigma_{a\sigma_a;\ b\sigma_b}\left(\omega\right)G_{b\sigma_b;\ j\sigma_j}\left(\omega\right),\\
W^{l\sigma_l;\ j\sigma_j}_{i\sigma_i;\ k\sigma_k}\left(\omega\right) &= v^{l\sigma_l;\ j\sigma_j}_{i\sigma_i;\ k\sigma_k} + v^{k\sigma_k;\ t\sigma_t}_{j\sigma_j;\ u\sigma_u}\tilde{P}^{x\sigma_x;\ y\sigma_y}_{u\sigma_u;\ t\sigma_t}\left(\omega\right)W^{l\sigma_l;\ x\sigma_x}_{i\sigma_i;\ y\sigma_y}\left(\omega\right).
\end{aligned} \tag{45}$$

Indeed, in the above equations we have turned all time integrals into products in frequency space, and only the contractions in the orbital indices remain. It is therefore computationally advantageous to evaluate these equations in frequency space, and Fourier transform to real time when needed. These are the equations we implemented in our code.

The interaction vertex $\Gamma$, as it appears in Hedin's equations, depends formally on three times. It is not obvious hence, *a priori*, whether a real frequency evaluation of the equations involving it is advantageous over the real time ones. We hence leave that as an open parameter, depending on the approximation. When giving the implementations below, we will give each one of the Hedin's equations in whatever axis (time or frequency) they are more efficiently evaluated. The equations for $G$ and $W$ remain unchanged throughout the approximations, and hence we do not repeat them below.

### A. sc$GW$

The $GW$ approximation is derived from the trivial (and most sever) approximation of the kernel $\frac{\delta\Sigma^{xc}}{\delta G} = \mathcal{K}_0 = 0$. From this, it follows $P = GG$, and $\Sigma^{xc} = iGW$ at each iteration. From this, we obtain a closed set of four Hedin's equations with Eq. (45) and

$$\begin{aligned}
\tilde{P}^{l\sigma_l;\ j\sigma_j}_{i\sigma_i;\ k\sigma_k}\left(t\right) &= -iG_{i\sigma_i;\ l\sigma_l}\left(-t\right)G_{j\sigma_j;\ k\sigma_k}\left(t\right),\\
\Sigma^{xc}{}_{i\sigma_i;\ j\sigma_j}\left(t\right) &= iG_{m\sigma_m;\ n\sigma_n}\left(t\right)W^{m\sigma_m;\ n\sigma_n}_{i\sigma_i;\ j\sigma_j}\left(t^+\right).
\end{aligned} \tag{46}$$

We note that unlike $W$ and $G$, the equations for $P$ and $\Sigma^{xc}$ are more efficiently evaluated in real time. We make use of the fast Fourier transform to change between both axes.

To reach self-consistency, hence sc$GW$, we iterate over Eq. (46) and (45) until the exchange-correlation self-energy stops changing (within some numerical threshold). For convergence purposes, sometimes we rely on the DIIS scheme [9, 10] for stability and to reduce the number of iterations.

### B. sc$GW\Gamma_G$

The next leading order approximation to the interaction kernel involves $\frac{\delta\Sigma^{xc}}{\delta G} = \mathcal{K}_0 + \mathcal{K}_G = \frac{\delta G}{\delta G}W\Gamma$, which to leading order becomes $\frac{\delta\Sigma^{xc}}{\delta G} \to v$. This leads to vertex corrections studied previously, in one-shot form, in Ref. [3–5]. This particularly simple form of the interaction kernel, particularly thanks to the trivial time structure of the bare Coulomb interaction $v$, allows us to write the interaction vertex as dependent of only one time/frequency variable. As a consequence, the equations for $\Gamma$, $P$ and $\Sigma^{xc}$ become

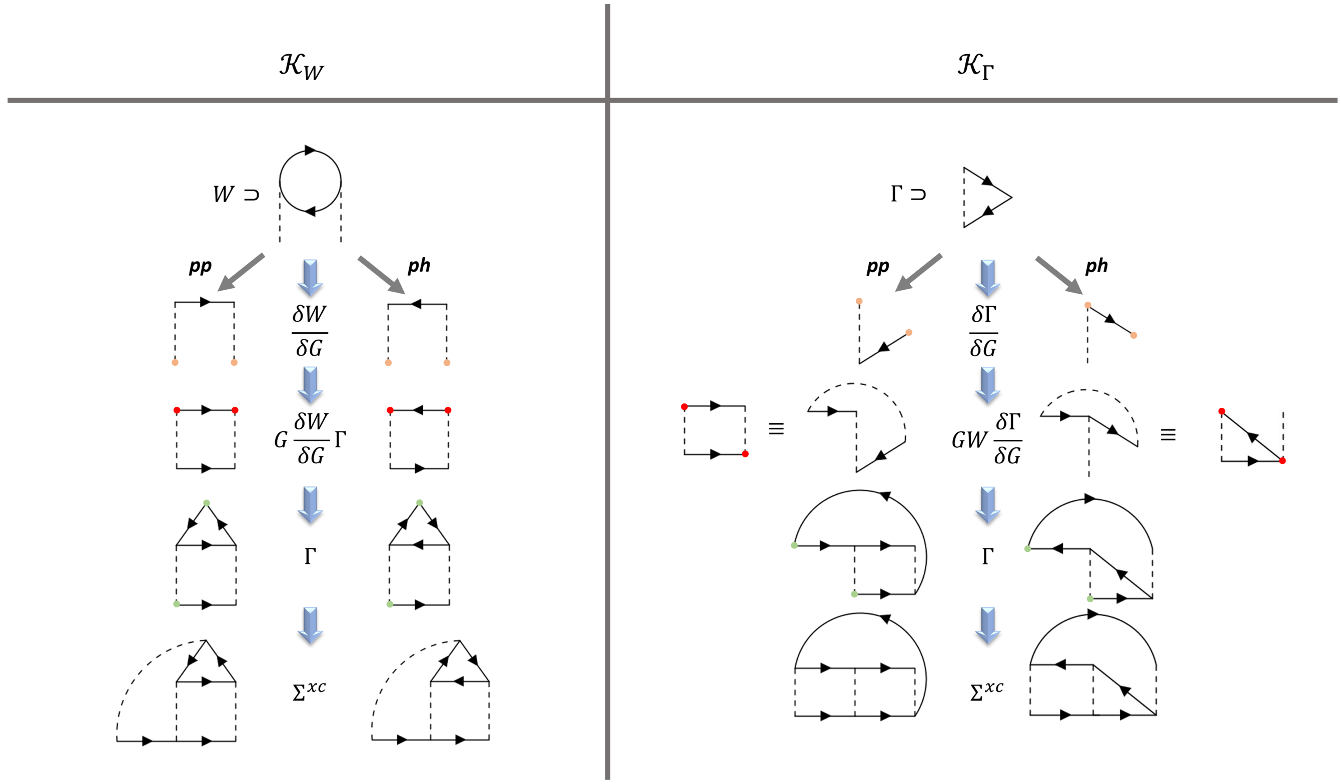


FIG. 3. Schematic of diagramatic derivation of the leading order contributions to $\Sigma^{xc}$ from $\mathcal{K}_W$ (left) and $\mathcal{K}_\Gamma$ (right). At each stage, the external legs on which subsequent diagramatic elements will be contracted are represented with dots. Starting from the lowest order term in $W$ or $\Gamma$ respectively, we show the effect of taking the functional derivative with respect to $G$ (in both the pp and ph channels), and the role of this functional derivative in $\mathcal{K}$, the corresponding contribution to the first order non-trivial term in $\Gamma$, and finally how this enters $\Sigma^{xc}$. See text for details.

$$
\begin{aligned}
\Gamma^{l\sigma_l;\, j\sigma_j}_{i\sigma_i;\, k\sigma_k}(\omega) &= \delta^{\sigma_i,\sigma_l}_{i,l}\,\delta^{\sigma_j,\sigma_k}_{j,k} + i v^{m\sigma_m;\, n\sigma_n}_{i\sigma_i;\, k\sigma_k}\,\tilde{P}^{RPA\ x\sigma_x;\, y\sigma_y}_{\quad\ m\sigma_m;\, n\sigma_n}(-\omega)\,\Gamma^{l\sigma_l;\, j\sigma_j}_{x\sigma_x;\, y\sigma_y}(\omega)\,,\\
\tilde{P}^{l\sigma_l;\, j\sigma_j}_{i\sigma_i;\, k\sigma_k}(\omega) &= \tilde{P}^{RPA\ m\sigma_m;\, n\sigma_n}_{\quad\ i\sigma_i;\, k\sigma_k}(\omega)\,\Gamma^{l\sigma_l;\, j\sigma_j}_{m\sigma_m;\, n\sigma_n}(-\omega)\,,\\
\Sigma^{xc}{}_{i\sigma_i;\, j\sigma_j}(t) &= iG_{m\sigma_m;\, n\sigma_n}(t)\,\Omega^{m\sigma_m;\, n\sigma_n}_{i\sigma_i;\, j\sigma_j}\left(t^+\right).
\end{aligned}
\tag{47}
$$

In the above equations, $\tilde{P}^{RPA}$ corresponds to the polarization in the RPA approximation, i.e. $\tilde{P} = -iGG$ as in Eq. (46), and we have introduced the auxiliary function

$$
\Omega^{l\sigma_l;\, j\sigma_j}_{i\sigma_i;\, k\sigma_k}(\omega) = W^{l\sigma_l;\, m\sigma_m}_{i\sigma_i;\, n\sigma_n}(\omega)\,\Gamma^{m\sigma_m;\, n\sigma_n}_{k\sigma_k;\, j\sigma_j}(-\omega)\,. \tag{48}
$$

Note that the polarization in this approximation only differs from the RPA approximation in the $GW$ implementation by a (frequency dependent) multiplicative factor $\Gamma$, hence the interaction vertex only enters the polarization as a convolution in real time. Similarly, the equation for the exchange-correlation self-energy is essentially the same as in $GW$, where the screened Coulomb interaction $W$ is substituted by an effective interaction $\Omega$ which is just a convolution in real time with $\Gamma$ away from $W$. It is meaningful to note, however, that this $W$ already contains $\Gamma$ through $P$, hence the vertex corrections enter $\Sigma^{xc}$ in two ways through $\Omega$. Similarly to our sc$GW$ implementation, we evaluate the five Hedin's equations here iteratively to self-consistency, resulting in our sc$GW\Gamma_G$ implementation. The one-shot version of this approach has been previously implemented in the real-space basis, c.f. Refs. [3–5].

### C. sc$GW\Gamma_G$ + $GW\Gamma_{W^{(1)}}$

The next leading order approximation to the interaction kernel involves $\frac{\delta\Sigma^{xc}}{\delta G} \supset \mathcal{K}_W = G\frac{\delta W}{\delta G}\Gamma$. We present a pictorial schematic of the derivation of its lowest order contribution in Fig. 3. This derives from the first non-trivial term in $W$ within the RPA approximation, namely the bubble $P^{RPA} \supset -iGG$ (see first line in the left side of Fig. 3. This generates two contributions of the type $\frac{\delta\Sigma^{xc}}{\delta G} \supset -ivGGv$, one in the particle-particle channel and the other in the particle-hole channel (see third line in the left side of Fig. 3). Ideally, this would be included in the Hedin equation for $\Gamma$ (c.f. Eq. (12)) *together* with the $\mathcal{K}_0$ and $\mathcal{K}_G$ contributions, and the resulting equation would be solved exactly. Unfortunately, the time structure of this equation does not correspond to a simple convolution, and hence we could not find a computationally low scaling approach to solve this equation accurately.

Instead, we opted for evaluating the first term in the exchange-correlation self-energy that derives from the $\mathcal{K}_W$ kernel, and add it to the $\Sigma^{xc}$ derived from the $GW\Gamma_G$ approximation in the last line of Eq. (47). These self-energy contributions correspond, in both pp and ph channels, to

$$\begin{aligned}
\tilde{\Sigma}^{xc,pp-W}{}_{i\sigma_i;\ l\sigma_l}(t) &= -i\tilde{T}^{pp-W}{}^{\ l\sigma_l;\ j\sigma_j}_{\ i\sigma_i;\ k\sigma_k}(t)\, G_{k\sigma_k;\ j\sigma_j}(-t)\,,\\
\tilde{\Sigma}^{xc,ph-W}{}_{i\sigma_i;\ l\sigma_l}(t) &= -i\tilde{T}^{ph-W}{}^{\ l\sigma_l;\ j\sigma_j}_{\ i\sigma_i;\ k\sigma_k}(t)\, G_{k\sigma_k;\ j\sigma_j}(t)\,,
\end{aligned} \tag{49}$$

where the superscript $pp-W/ph-W$ denotes the pp and ph channels as derived from the $\mathcal{K}_W$ kernel (c.f. final line in the left panel of Fig. 3). The tilde denotes that this is a first order (non-resummed) approximation, as discussed above. The $T$ operators encode the $vGGvGGv$ box corresponding to the first terms in the direct $T$-matrix approximation, and can be evaluated in frequency space as

$$\begin{aligned}
\tilde{T}^{pp-W}{}^{\ l\sigma_l;\ j\sigma_j}_{\ i\sigma_i;\ k\sigma_k}(\omega) &= -v^{x\sigma_x;\ j\sigma_j}_{i\sigma_i;\ y\sigma_y}\Theta^{pp}{}^{\ n\sigma_n;\ y\sigma_y}_{\ x\sigma_x;\ m\sigma_m}(\omega)\,\Theta^{pp}{}^{\ l\sigma_l;\ m\sigma_m}_{\ n\sigma_n;\ k\sigma_k}(\omega)\,,\\
\tilde{T}^{ph-W}{}^{\ l\sigma_l;\ j\sigma_j}_{\ i\sigma_i;\ k\sigma_k}(\omega) &= v^{x\sigma_x;\ y\sigma_y}_{i\sigma_i;\ k\sigma_k}\Theta^{ph}{}^{\ n\sigma_n;\ m\sigma_m}_{\ x\sigma_x;\ y\sigma_y}(\omega)\,\Theta^{ph}{}^{\ l\sigma_l;\ j\sigma_j}_{\ n\sigma_n;\ m\sigma_m}(\omega)\,.
\end{aligned} \tag{50}$$

Finally, the auxiliary operators $\Theta$ encode the building unit $vGG$ with which to form the full $T$-matrix "boxes", and they follow (in real time)

$$\begin{aligned}
\Theta^{pp}{}^{\ x\sigma_x;\ y\sigma_y}_{\ n\sigma_n;\ p\sigma_p}(t) &= iG_{n\sigma_n;\ q\sigma_q}(t)\, v^{x\sigma_x;\ r\sigma_r}_{q\sigma_q;\ p\sigma_p}G_{y\sigma_y;\ r\sigma_r}(t)\,,\\
\Theta^{ph}{}^{\ x\sigma_x;\ y\sigma_y}_{\ n\sigma_n;\ p\sigma_p}(t) &= -iG_{n\sigma_n;\ q\sigma_q}(t)\, v^{x\sigma_x;\ y\sigma_y}_{q\sigma_q;\ r\sigma_r}G_{r\sigma_r;\ p\sigma_p}(-t)\,.
\end{aligned} \tag{51}$$

As we see, all steps in this approximation can be evaluated as time or frequency products, involving only contractions in orbital space but no integrals. This is due to the convolutional time-structure in the leading term contribution of $\mathcal{K}_W$ to the interaction vertex $\Gamma$, which unfortunately does not carry on to the full resummation that would appear in Eq. (12). This convolutional structure does however carry on to the higher order $T$-matrix like terms, and this is what will allow us to perform the selected self-consistency in the sc$GW\Gamma_G + GW\Gamma_{W,\Gamma}$ method below, essentially resumming the full $T$-matrix expansion.

We note that including the $\tilde{\Sigma}^{xc,pp-W}$ and $\tilde{\Sigma}^{xc,ph-W}$ terms within the self-consistent (iterative) evaluation of Hedin's equations greatly reduced the stability of the iterations, precluding proper convergence. Hence, we opted instead for a one-shot correction after converging a sc$GW\Gamma_G$ calculation, using the fully dressed Green's functions obtained from sc$GW\Gamma_G$ in Eq. (49)-(51). We denote this method therefore as sc$GW\Gamma_G + GW\Gamma_{W^{(1)}}$.

### D. sc$GW\Gamma_G$ + $GW\Gamma_{W^{(1)},\Gamma^{(2)}}$

The final, qualitatively distinct approximation we introduce in this work involves including to lowest order the last interaction kernel, i.e. the functional derivative of the interaction vertex itself with respect to the Green's function $\frac{\delta\Sigma^{xc}}{\delta G} \supset \mathcal{K}_\Gamma = GW\frac{\delta\Gamma}{\delta G}$. This term is noteworthy on two accounts: on the one hand, it has been neglected in all previous work (to the best of our knowledge), and on the other hand it is the term responsible for introducing qualitatively distinct diagrams through the iteration of Hedin's equations, as motivated in the main paper. As a consequence of this latter fact, it can allow the application of Hedin-based perturbation theory beyond the weakly interacting (highly screened) limit, as we exemplify on the simple Hubbard dimer in our work. This can be both qualitative (in the leading order implementations of the self-energy contributions of $\mathcal{K}_\Gamma$), as well as quantitative (when including at least some degree of self-consistency, as in the resummation of the full $T$-matrix channels).

In this subsection, we consider only the lowest order contribution of $-$. A schematic representation of the derivation of this lowest order terms is given in the right side of Fig. 3. This is done in complete analogy to the $\mathcal{K}_W$ contributions presented in the previous subsection. First of all, we consider only the leading order, non-trivial component of $\Gamma$ inside the functional derivative (c.f. first line in the right side of Fig. 3). This corresponds to the first term in Eq. (47), proportional to $\Gamma \supset vGG$. Upon taking the functional derivative of this term with respect to $G$ (c.f. second line in the right side of Fig. 3), and contracting with the leading order $GW \to Gv$, we end with two contributions of the type $\frac{\delta\Sigma^{xc}}{\delta G} \supset -ivGGv$ (see third line of the right side in Fig. 3). These are completely analogous to the terms arising from $\mathcal{K}_W$, however with a different orbital contraction order. As a consequence, while the $W$-kernel generates to leading order the initial terms in the *direct* $T$-matrix expansion in the pp and ph channels, the first order $\Gamma$-kernel contributions are the corresponding *exchange* $T$-matrix expansion diagrams (c.f. final line on the right side of Fig. 3). Just as it is the case in the $\mathcal{K}_W$ components, the time structure of the $\frac{\delta\Sigma^{xc}}{\delta G}$ contribution from $\mathcal{K}_\Gamma$ precludes us from finding a simple closed expression for $\Gamma$ which includes the full resummation of diagrams while being computationally tractable. Hence, we opt instead for evaluating the contribution of the leading order term of $\mathcal{K}_\Gamma$ directly on the exchange correlation self-energy, for both the pp and ph channels. These contributions were then added to the fully resummed exchange-correlation self-energy of the sc$GW\Gamma_G$ approximation. We evaluate these contributions following

$$\begin{aligned}
\tilde{\Sigma}^{xc,pp-\Gamma}{}_{i\sigma_i;\ k\sigma_k}(t) &= i\tilde{T}^{pp-W}{}^{\ l\sigma_l;\ j\sigma_j}_{\ i\sigma_i;\ k\sigma_k}(t)\, G_{l\sigma_l;\ j\sigma_j}(-t)\,,\\
\tilde{\Sigma}^{xc,ph-\Gamma}{}_{i\sigma_i;\ k\sigma_k}(t) &= \tilde{T}^{ph-\Gamma}{}^{\ l\sigma_l;\ j\sigma_j}_{\ i\sigma_i;\ k\sigma_k}(t)\, G_{l\sigma_l;\ j\sigma_j}(t)\,,
\end{aligned} \tag{52}$$

where, consistently with the previous subsection, the superscript $pp-\Gamma/ph-\Gamma$ denotes the pp and ph channels as derived from the $\mathcal{K}_\Gamma$ kernel. The tilde denotes that this is a first order (non-resummed) approximation, as discussed above. The $T$ operators encode the $vGGvGGv$ box corresponding to the first terms in the exchange $T$-matrix approximation. For the pp channel, this coincides with the $T$ operator derived from the $\mathcal{K}_W$ contribution, but this is not the case in the ph channel. Evaluating $\tilde{T}^{ph-\Gamma}$ instead involves

$$\begin{aligned}
\tilde{T}^{ph-\Gamma}{}^{\ l\sigma_l;\ j\sigma_j}_{\ i\sigma_i;\ k\sigma_k}(\omega) &= \tilde{T}^{ph-\Gamma-2}{}^{\ m\sigma_m;\ n\sigma_n}_{\ i\sigma_i;\ l\sigma_l}(\omega)\, \tilde{\Theta}^{ph,2}{}^{\ n\sigma_n;\ j\sigma_j}_{\ m\sigma_m;\ k\sigma_k}(\omega)\,,\\
\Theta^{ph,2}{}^{\ l\sigma_l;\ j\sigma_j}_{\ i\sigma_i;\ k\sigma_k}(t) &= G_{i\sigma_i;\ n\sigma_n}(-t)\, G_{m\sigma_m;\ l\sigma_l}(t)\, v^{m\sigma_m;\ j\sigma_j}_{n\sigma_n;\ k\sigma_k}\,,\\
\tilde{T}^{ph-\Gamma-2}{}^{\ l\sigma_l;\ j\sigma_j}_{\ i\sigma_i;\ k\sigma_k}(\omega) &= v^{x\sigma_x;\ y\sigma_y}_{i\sigma_i;\ k\sigma_k}\, \Theta^{ph}{}^{\ l\sigma_l;\ j\sigma_j}_{\ x\sigma_x;\ y\sigma_y}(\omega)\,.
\end{aligned} \tag{53}$$

As above, the auxiliary operators $\Theta$ encode the building unit $vGG$ with which to form the full $T$-matrix "boxes", and they follow the same relations defined in the previous subsection, c.f. Eq. (51), except for the new operator $\Theta^{ph,2}$.

We appreciate the analogy between the terms derived from the $\mathcal{K}_\Gamma$ and $\mathcal{K}_W$ kernels, distinguished only by the order of orbital contractions, which motivates their identification as exchange and direct components correspondingly. As was the case with the $\mathcal{K}_W$ contributions, we do not include the self-energy terms in Eq. (52) within the self-consistent iteration through Hedin's equations, but instead add them as one-shot correction on top of a self-consistently converged sc$GW\Gamma_G$ calculation, using the converged (hence fully dressed) Green's function. Addind this and the contribution from $\mathcal{K}_W$ gives rise to our sc$GW\Gamma_G + GW\Gamma_{W^{(1)},\Gamma^{(2)}}$ implementation. The superindices (1) and (2) indicate that the $\mathcal{K}_W$ terms would arise in the first iteration after $GW$, while the $\mathcal{K}_\Gamma$ contributions would appear at the second iteration after $GW$.

### E. sc$GW\Gamma_G$ + $GW\Gamma_{W,\Gamma}$

Finally, we implement a perturbative approximation that accounts for some of the self-consistency that is missing in the previous leading order approximations to the $\mathcal{K}_W$ and $\mathcal{K}_\Gamma$ contributions. As discussed above, there are forms of self-consistency that we were not able to express in a closed, computationally tractable way. For example, the resummation in the full evaluation of the Dyson-like equation for $\Gamma$ (c.f. Eq. (12)) falls under this category. As a consequence, we are missing some of the "screening" of the diagrams included in $\Gamma$, likely overestimating their contribution. By comarison with the analogous situation in the Dyson-like equation for $W$, or indeed the difference between one-shot $G_0W_0$ and sc$GW$, it seems reasonable to expect that the neglected terms will only account for some degree of quantitative disagreement with the true Green's function of the system, but will not cause a qualitative error in our calculation.

However, other forms of self-consistency can very well account for qualitative discrepancies with the true Green's function. Indeed, in the main paper we argue and exemplify that this is exactly the effect of $\mathcal{K}_\Gamma \supset \frac{\delta\Gamma}{\delta G}$, which in each iteration through Hedin's equations will generate topologically distinct diagrams to those previously encountered[11].

This special role of $\frac{\delta\Gamma}{\delta G}$ becomes also apparent in the general expression for $\frac{\delta W}{\delta G}$ that appears in $\mathcal{K}_W$, as in the first subsection of the SI. We can account for some of these topologically disitinct contributions from $\mathcal{K}_\Gamma$, hence expanding the validity of the Hedin-based perturbative expansion beyond the weakly-interacting regime, as shown for the Hubbard dimer in the main body of the paper. To be specific, we perform the full $T$-matrix expansion resumation, the first order terms of which are given by the $GW\Gamma_{W^{(1)},\Gamma^{(2)}}$ approximation described above. As we show in the main paper, each successive diagram of the $T$-matrix resummation is arises from the action of the functional derivative with respect to $G$ of the diagram in $\Gamma$ corresponding to the preceding term in the expansion. In other words, the full $T$-matrix expansion can be recovered, order-by-order within Hedin's formalism, collecting a new term at each iteration through the equations.

We implement this resummation by rewriting the equations for the $\tilde{T}^W$ terms in Eq. (50) and the $\tilde{T}^{\Gamma-2}$ term inn Eq. (53) (keeping the equation for $\tilde{T}^{ph-\Gamma}$ as is) into Dyson-like equations, involving full resummations of the interaction boxes. These follow

$$\begin{aligned}
T^{pp-W}\,{}^{l\sigma_l;\; j\sigma_j}_{i\sigma_i;\; k\sigma_k}(\omega) &= v^{x\sigma_x;\; j\sigma_j}_{i\sigma_i;\; y\sigma_y}\,\Theta^{pp}\,{}^{m\sigma_m;\; y\sigma_y}_{x\sigma_x;\; n\sigma_n}(\omega)\,\Theta^{pp}\,{}^{l\sigma_l;\; n\sigma_n}_{m\sigma_m;\; k\sigma_k}(\omega) - T^{pp-W}\,{}^{x\sigma_x;\; j\sigma_j}_{i\sigma_i;\; y\sigma_y}(\omega)\,\Theta^{pp}\,{}^{l\sigma_l;\; y\sigma_y}_{x\sigma_x;\; k\sigma_k}(\omega)\,,\\
T^{ph-W}\,{}^{l\sigma_l;\; j\sigma_j}_{i\sigma_i;\; k\sigma_k}(\omega) &= v^{x\sigma_x;\; y\sigma_y}_{i\sigma_i;\; k\sigma_k}\,\Theta^{ph}\,{}^{m\sigma_m;\; n\sigma_n}_{x\sigma_x;\; y\sigma_y}(\omega)\,\Theta^{ph}\,{}^{l\sigma_l;\; j\sigma_j}_{m\sigma_m;\; n\sigma_n}(\omega) + T^{ph-W}\,{}^{x\sigma_x;\; y\sigma_y}_{i\sigma_i;\; k\sigma_k}(\omega)\,\Theta^{ph}\,{}^{l\sigma_l;\; j\sigma_j}_{x\sigma_x;\; y\sigma_y}(\omega)\,,\\
T^{ph-\Gamma-2}\,{}^{l\sigma_l;\; j\sigma_j}_{i\sigma_i;\; k\sigma_k}(\omega) &= v^{x\sigma_x;\; y\sigma_y}_{i\sigma_i;\; k\sigma_k}\,\Theta^{ph}\,{}^{l\sigma_l;\; j\sigma_j}_{x\sigma_x;\; y\sigma_y}(\omega) + T^{ph-\Gamma-2}\,{}^{x\sigma_x;\; y\sigma_y}_{i\sigma_i;\; k\sigma_k}(\omega)\,\Theta^{ph}\,{}^{l\sigma_l;\; j\sigma_j}_{x\sigma_x;\; y\sigma_y}(\omega)\,.
\end{aligned} \tag{54}$$

The contributions to the exchange-correlation self-energy then follow Eq. (49) and (52), with the $\tilde{T}$ operators substituted by the fully resumed $T$ operators. As with all contributions from $\mathcal{K}_W$ and $\mathcal{K}_\Gamma$, we add the contributions to $\Sigma^{xc}$ coming from the resummed $T$-matrix expressions as a one-shot correction to the self-consistently converged sc$GW\Gamma_G$ self-energy. This is the sc$GW\Gamma_G + GW\Gamma_{W,\Gamma}$ approximation used in the main paper.

## IV. MEAN FIELD THEORY OF THE HUBBARD DIMER

In this subsection, we will give a brief recount on the mean-field theory of the Hubbard dimer at half-filling, its ground state energy and single particle gap, particularly with focus on spatial translational symmetry broken vs symmetric solution.

The Hamiltonian of the Hubbard dimer follows:

$$H_{dimer} = -t \sum_{\sigma\in\{\uparrow,\downarrow\}} \left(c^\dagger_{1,\sigma}c_{2,\sigma} + \text{c.c.}\right) + U\sum_{i=1}^{2} n_{i,\uparrow}n_{i,\downarrow} + \mu\sum_{i,\sigma} n_{i,\sigma}, \tag{55}$$

with hopping amplitude $t$, Coulomb repulsion $U$, and chemical potential $\mu$. At half-filling, particle-hole symmetry fixes $\mu = -U/2$. We can evaluate this Hamiltonian within mean-field theory by writing the spin-dependent particle number operators as their average $\langle n_{i,\sigma}\rangle$ plus fluctuation $\delta n_{i,\sigma}$

$$n_{i,\sigma} = \langle n_{i,\sigma}\rangle + \delta n_{i,\sigma}. \tag{56}$$

With this decomposition, we can evaluate the interaction term $Un_{i,\uparrow}n_{i,\downarrow}$ within mean-field theory, i.e. neglecting second order terms in the fluctuation, and after some standard manipulations arrive at

$$H^{MF}_{dimer} = -t \sum_{\sigma\in\{\uparrow,\downarrow\}} \left(c^\dagger_{1,\sigma}c_{2,\sigma} + \text{c.c.}\right) + U\sum_{i=1}^{2} \left[n_{i,\uparrow}\langle n_{i,\downarrow}\rangle + \langle n_{i,\uparrow}\rangle n_{i,\downarrow}\right] - U\sum_{i=1}^{2}\langle n_{i,\uparrow}\rangle\langle n_{i,\downarrow}\rangle + \mu\sum_{i,\sigma} n_{i,\sigma}. \tag{57}$$

Now, we will concentrate on solutions with tranlational symmetric charge density but potentially translational symmetry breaking spin density. In particular, we will allow for opposite magnetizations on the two sites of the dimer. To account for these possible solutions, we can parametrize the average spin-charge densities as

$$\begin{aligned}
n &\equiv \langle n_{i,\uparrow}\rangle + \langle n_{i,\downarrow}\rangle,\\
m &\equiv (-1)^i \left(\langle n_{i,\uparrow}\rangle - \langle n_{i,\downarrow}\rangle\right).
\end{aligned} \tag{58}$$

| | Exact | Symm. MF | Symm. Broken MF $U/t > 2$ |
|---|---|---|---|
| Ground state energy $E_0$ | $-\frac{U}{2}(1+\sqrt{1+(\frac{4t}{U})^2})$ | $-2t-\frac{U}{2}$ | $-U-\frac{2t^2}{U}$ |
| $\lim_{U/t\to\infty} E_0$ | $-U-\frac{4t^2}{U}$ | $-2t-\frac{U}{2}$ | $-U-\frac{2t^2}{U}$ |
| Single quasiparticle gap $\Delta$ | $2t\sqrt{4+\frac{U}{2t}}-2t$ | $2t$ | $U$ |
| $\lim_{U/t\to\infty} \Delta$ | $U+\frac{8t^2}{U}-2t$ | $2t$ | $U$ |

TABLE I. Ground state energy $E_0$ and single quasiparticle gap $\Delta$, with their respective asymptotic behaviors for $U/t \to \infty$ in the Hubbard dimer at half-filling. Compared are the exact solution with the symmetric and symmetry broken mean-field discussed in the text. Note that for $U/t < 2$ the mean-field does not break translational symmetry

Note that imposing translational invariance in the charge density implies $n = \frac{N_{el}}{N_{sites}}$. With this parametrization, the mean-field Hamiltonian can be simplified to

$$H^{MF}_{dimer} = -t \sum_{\sigma\in\{\uparrow,\downarrow\}} \left(c^\dagger_{1,\sigma}c_{2,\sigma} + \text{c.c.}\right) + \frac{U}{2}m\sum_{i=1}^{2}(-1)^i\left[n_{i,\downarrow} - n_{i,\uparrow}\right] - \frac{U}{2}\left[1-m^2\right]. \tag{59}$$

To arrive at this result, we have used $\mu = -U/2$ as well as $n = 1$ at half-filling. From this, t follows that the ground state energy for a dimer with 1 electron of spin up and 1 electron of spin up as a function of the local magnetization $m$ is

$$E_0^{1\uparrow,1\downarrow}(m) = -2t\sqrt{1+m^2\left(\frac{U}{2t}\right)^2} - \frac{U}{2} + \frac{U}{2}m^2. \tag{60}$$

The variational principle allows us then to obtain the ground state magnetization $m$ as a function of $U$ as

$$m(U) = \begin{cases} 0 & U \leq 2t \\ \pm\sqrt{1-\left(\frac{2t}{U}\right)^2} & U \geq 2t \end{cases}, \tag{61}$$

which follows a behavior not unlike the spin magnetization of the Ising model in mean-field theory. In a sense, this change of behavior in the mean-field solution at $U = 2t$, from non-magnetic to antiferromagnetic, identifies $U = 2t$ as a region of "strong correlation" in the $U/t$ phase diagram. It is in this regard that we consider the regime $U/t > 2$ as the high-interaction regime, and the $U/t < 2$ as the weak interaction regime.

We turn now to some basic properties of the spatial translation symmetric ($m = 0$) and symmetry broken ($m \neq 0$) solutions, in comparison with the exact result. Tab. I summarizes the ground state energy, and its asymptotic behavior at $U/t \to \infty$ for the three cases. For $U/t < 2$ both mean-field solutions coincide, and they give the right asymptotic ground state in the $U/t \to 0$ limit. The difference lies thus in the $U/t \to \infty$ limit. Here, we see that the departure from the symmetric mean-field solution from the exact one diverges as $U$, while the symmetry broken solution presents the right $\frac{t^2}{U}$. Notably, the prefactor is only half as large as the exact one, since there are two degenerate symmetry broken solutions, while the true ground state is symmetric. To recover the exact prefactor (and hence the exact ground state energy) in the high interaction limit is still possible within degenerate perturbation theory, treating $\frac{t^2}{U}$ as the small perturbative energy scale. Similar to the total ground state energy, we can evaluate the single quasiparticle gap $\Delta$, corresponding to the energy difference between the main quasiparticle hole and particle peaks in the one-body Green's functions. We see that the symmetric mean-field presents an interaction strength independent gap of $2t$, while the symmetry-broken mean-field given an exactly linear gap $U$. While none of them give the exact asymptotic behavior for large interactions, the symmetry broken mean-field can reproduce the leading order term in the exact result.

From these energetic considerations, using the symmetry broken mean-field is a clearly more attractive initial guess for any perturbative treatment in the high $U$ limit, where the perturbative energy scale would be $t^2/U$. We attempted this in the main text, using the symmetry-broken mean-field solution presented here as initial step in our MBPT calculations. However, since all our diagrams preserve the spin-projection on the $z$ axis, i.e. we did not account for any spin-flip processes, our simulations were not able recover the symmetry even at self-consistency. Further, we observed little to no improvement of the symmetry-broken mean-field results on the large $U/t$ limit with any of our perturbative approximations, suggesting that within the space of symmetry broken solutions (accessible through perturbation theory), the mean-field starting point is already the best possible solution. Exploring perturbative

approaches accounting for spin-flip processes, and hence potentially capable of recovering the symmetric solution at self-consistency, remains an interesting avenue of investigation. By analogy with degenerate perturbation theory for the simple Hubbard dimer, which becomes exact in the high $U/t$ limit, this may prove a very successful alternative for perturbative expansions.

## V. SIMULATION PARAMETERS

Finally, in this subsection we collect the technical simulation parameters that we used to generate the data represented in the main paper.

We used the half-filled Hubbard dimer (c.f. Eq. (55)) to test our different perturbative approaches. The hopping amplitude $t$ served as our energy unit, and hence we set $t \equiv 1$, and used the Coulomb repulsion $U/t$ as our free parameter to explore the weakly and strongly interacting regimes. At half-filling, the chemical potential is fixed at $\mu = -U/2$.

To sample the frequency/time dependent operators, we used a frequency grid of $N_\omega \sim 2^{20}$ points, in a span from $[-400\ t, 400\ t]$, giving a frequency spacing of $\Delta\omega \approx 0.01\ t$. The actual number of grid points was given by scipy's next_fast_len routine in the fast Fourier transform (fft) package. The time grid is fixed then by the condition $N_\omega = N_t$ and $\Delta\omega * \Delta t = 2\pi/N_\omega$. We used an artificial broadening factor of $\eta = 0.01\ t$ for all magnitudes in frequency space, which corresponds to a exponential dampening factor in real time.

Within the iterative procedure, we implemented a simple DIIS update for the exchange-correlation self-energy, taking into account the last 3 iterations. We observed most our calculations to converge within 20 iterations, those that did not often presented oscillatory behavior and could not ultimatively be converged. These had all started from the symmetry broken mean-field in the intermediate $U$ regime, and are represented by transparent markers in Fig. 3 of the main paper.

---


[1] L. Hedin, New method for calculating the one-particle green's function with application to the electron-gas problem, Phys. Rev. **139**, A796 (1965).

[2] R. M. Martin, L. Reining, and D. M. Ceperley, *Interacting Electrons: Theory and Computational Approaches* (Cambridge University Press, 2016).

[3] E. Maggio and G. Kresse, GW vertex corrected calculations for molecular systems, J. Chem. Theory Comput. **13**, 4765 (2017).

[4] V. Vlček, Stochastic vertex corrections: Linear scaling methods for accurate quasiparticle energies, J. Chem. Theory Comput. **15**, 6254 (2019).

[5] C. Mejuto-Zaera, G. Weng, M. Romanova, S. J. Cotton, K. B. Whaley, N. M. Tubman, and V. Vlček, Communication: Are multi-quasiparticle interactions important in molecular ionization?, J. Chem. Phys. **154**, 121101 (2021).

[6] R. D. Sole, L. Reining, and R. W. Godby, $GW\Gamma$ approximation for electron self-energies in semiconductors and insulators, Phys. Rev. B **49**, 8024 (1994).

[7] Involving the trivial relation $\frac{\partial}{\partial u}\left[GG^{-1}\right] = 0$.

[8] Abusing a bit the language of variable transformations.

[9] P. Pulay, Convergence acceleration of iterative sequences. the case of scf iteration, Chem. Phys. Lett. **73**, 393 (1980).

[10] P. Pulay, Improved scf convergence acceleration, J. Comp. Chem. **3**, 556 (1982).

[11] This means, diagrams that cannot be reduced to previous diagrams by substituting bare propagator or interaction lines for dressed ones.
